# Supplementary material for: Benchmarking Visual Localization for Autonomous Navigation
Source: arXiv:2203.13048 source file (2022-10-18)
Supplement: Supplementary file 1 [file supplementary.tex]

% For each experiment:
%   - Failure rate plot
%   - Failure rate table
%   - Recall table
%   - Recall vs failure rate plot

% Illumination - Town01
\begin{table*}[!t]
\section{Additional experiment results}
\label{sec:appendix}

This appendix includes the full set of results for each experiment type: illumination change, viewpoint change and weather change. For each experiment, we show \vspace{0.1cm}

\textbf{1)} Plot of failure rate vs. the main experiment parameter;

\textbf{2)} Correlation plot of the failure and recall rates;

\textbf{3)} Table of the failure rates for each value of the main experiment parameter;

\textbf{4)} Table of the recall rates measured by driving the route by autopilot with access to ground truth vehicle state;
\vspace{0.2cm}

For the illumination change we show results from two environments (Town01 and Town10). The viewpoint experiments were conducted only in Town01, the weather experiments in Town10. For full experiment specifications see the main paper.

\subsection{Illumination change results - Town01}
%\hfill%
\begin{minipage}[t]{0.48\linewidth}
  \centering
  \begin{adjustbox}{width=\linewidth, valign=T}
   \includegraphics[width=1.0\linewidth, trim={0 1cm 0cm 1cm}]{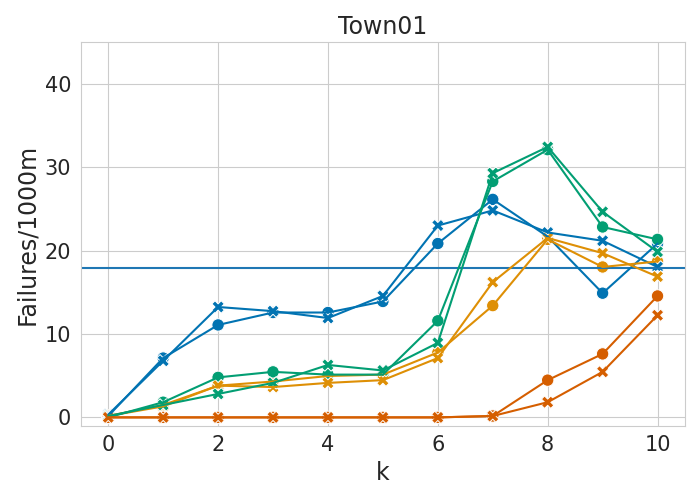}
   \end{adjustbox}
   \captionof{figure}{ Relationship of failure rate with illumination levels $k$. Marker color indicates type for local features, shape for global features.}
   \label{fig:supplementary_fr_kvalue_correlation}
\end{minipage}%
\hfill
\begin{minipage}[t]{0.48\linewidth}
  \centering
  \begin{adjustbox}{width=\linewidth, valign=T}
   \includegraphics[width=1.0\linewidth, trim={0 1cm 0cm 1cm}]{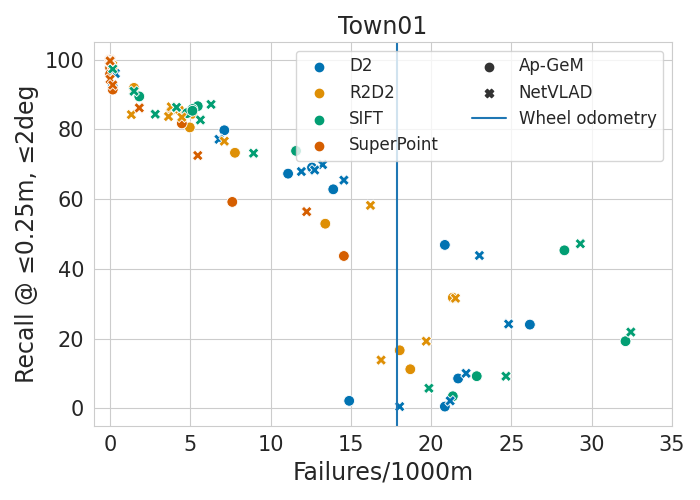}
   \end{adjustbox}
   \captionof{figure}{ Relationship between the failure rate and recall rate T1. Marker color and shape indicate feature type.}
   \label{fig:supplementary_illumination_fr_recall_correlation}
   \vspace{0.5cm}
\end{minipage}
\vspace{0.5cm}
\hfill
\begin{minipage}[t]{0.75\linewidth}
      \centering
  \resizebox{0.90\linewidth}{!}{
  \begin{tabular}{l l r r r r r r r r r r r r  }
  &  & \multicolumn{11}{c}{Town01}       \\
    \cmidrule(lr){3-13}
    %\midrule
         % town01
     PR & LF &  $k=$ 0 & 1 & 2 & 3 & 4 & 5 & 6 & 7 & 8 & 9 & 10 
     \\
    %\midrule
    \midrule
     % town01
    Ap- & Sift  & \textbf{0.0} & 1.8 & 4.8 & 5.5 & 5.1 & 5.1 & 11.6 & 28.3 & 32.1 & 22.8 & 21.4 
    \\
     % town01
     GeM & D2-net  & 0.2 & 7.1 & 11.1 & 12.6 & 12.6 & 13.9 & 20.9 & 26.2 & 21.7 & 14.9 & 20.9
     \\
      % town01
     & R2D2  & 0.2 & 1.5 & 3.8 & 4.3 & 5.0 & 5.1 & 7.8 & 13.4 & 21.4 & 18.0 & 18.7
     \\
     % town01
     & SuperPoint & \textbf{0.0} & \textbf{0.0} & \textbf{0.0} & \textbf{0.0} & \textbf{0.0} & \textbf{0.0} & \textbf{0.0} & \textbf{0.2} & 4.5 & 7.6 & 14.6
     \\
    \midrule
     % town01
    Net- & Sift  & 0.2 & 1.5 & 2.8 & 4.1 & 6.3 & 5.6 & 8.9 & 29.3 & 32.5 & 24.7 & 19.9
    \\
     % town01
     VLAD & D2-net  & 0.3 & 6.8 & 13.2 & 12.7 & 11.9 & 14.6 & 23.0 & 24.8 & 22.2 & 21.2 & 18.0
    \\
    %town01
     & R2D2  & 0.2 & 1.3 & 3.8 & 3.6 & 4.1 & 4.5 & 7.1 & 16.2 & 21.5 & 19.7 & 16.9
     \\
     %town01
     & SuperPoint  & \textbf{0.0} & \textbf{0.0} & \textbf{0.0} & \textbf{0.0} & \textbf{0.0} & \textbf{0.0} & \textbf{0.0} & \textbf{0.2} & \textbf{1.8} & \textbf{5.5} & \textbf{12.3}
     \\
     \midrule
     \multicolumn{2}{l}{Wheel odometry} &  \multicolumn{11}{c}{17.9}
      \\
     \bottomrule
  \end{tabular}
  }
    \caption{Navigation failure rates over 5 repeated runs of the same route at each illumination level $k$. Smaller is better. PR $=$ place recognition method, LF $=$ local feature type.}
    \label{tab:supplementary_failure_illumination_town01}
    \end{minipage}
    \hfill
    \vspace{0.5cm}
\begin{minipage}[t]{\linewidth}
\newcommand\mcat{T1 / T2 / T3}

%\tiny
  \centering
  \resizebox{1.0\linewidth}{!}{
  \begin{tabular}{c c  c c c c c c c c c c c c c c c c c}
  & & \multicolumn{11}{c}{Town01}   \\
    \cmidrule{3-13}
    \vspace{-0.45cm}
    \\
    \cmidrule{3-13}
     \multirow{2}{*}{PR} & \multirow{2}{*}{LF} &  $k=$ 0 & 1 & 2 & 3 & 4 & 5 & 6 & 7 & 8 & 9 & 10 \\
    \cmidrule{3-13}
    & &   \mcat\  & \mcat\  & \mcat\ & \mcat\ & \mcat\ & \mcat\ & \mcat\ & \mcat\ & \mcat\ & \mcat\ & \mcat\  \\
    %& &   \dcat\ & \dcat\ & \dcat\ & \dcat\ & \dcat\ & \dcat\ & \dcat\ & \dcat\ & \dcat\ & \dcat\ & \dcat\  \\
    \midrule
    Ap- & Sift  & 98.0 / 98.2 / 99.8 & 89.5 / 92.9 / 99.0 & 84.7 / 89.6 / 96.5 & 86.7 / 89.3 / 96.1 & 85.9 / 89.3 / 96.7 & 85.4 / 89.5 / 95.4 & 73.8 / 78.5 / 90.5 & 45.3 / 51.6 / 63.9 & 19.2 / 23.8 / 29.8 & 9.2 / 11.8 / 16.4 & 3.5 / 5.8 / 8.6  \\
    
     GeM & D2-net   & 92.3 / 95.7 / 99.8 & 79.8 / 86.7 / 97.5 & 67.3 / 74.7 / 90.1 & 68.8 / 74.8 / 90.1 & 69.1 / 74.7 / 88.0 & 62.8 / 70.9 / 85.7 & 46.9 / 58.1 / 73.8 & 24.0 / 28.5 / 39.3 & 8.6 / 10.9 / 15.6 & 2.1 / 3.1 / 6.2 & 0.5 / 0.8 / 2.0  \\
     
     & R2D2   & 98.0 / 98.4 / \textbf{100.0} & 91.9 / 94.1 / 98.7 & 85.5 / 90.4 / 97.7 & 85.7 / 90.6 / 96.2 & 80.6 / 88.2 / 97.0 & 84.5 / 88.0 / 96.5 & 73.3 / 79.7 / 93.6 & 53.0 / 62.8 / 79.1 & 31.7 / 37.5 / 50.5 & 16.6 / 20.4 / 23.6 & 11.2 / 12.9 / 15.0 \\
     
     & SuperPoint  &  \textbf{100.0} / \textbf{100.0} / \textbf{100.0} & \textbf{100.0} / \textbf{100.0} / \textbf{100.0} & \textbf{99.8} / \textbf{99.8} / 99.8 & 97.7 / 99.8 / \textbf{100.0} & 99.5 / \textbf{100.0} / \textbf{100.0} & 99.2 / 99.3 / 99.7 & \textbf{95.9} / 98.5 / 99.0 & 91.4 / 94.6 / 96.5 & 81.7 / 86.3 / 90.5 & 59.2 / 65.0 / 71.5 & 43.7 / 48.9 / 57.9 \\
   \midrule
    Net- & Sift   & 97.4 / 98.5 / 99.8 & 91.0 / 93.3 / 99.2 & 84.4 / 87.7 / 97.5 & 86.3 / 89.5 / 96.9 & 87.2 / 89.8 / 97.4 & 82.7 / 87.5 / 96.5 & 73.2 / 79.6 / 92.3 & 47.2 / 53.1 / 67.6 & 21.9 / 27.0 / 34.4 & 9.2 / 13.8 / 20.5 & 5.8 / 8.2 / 13.0   \\
    
     VLAD & D2-net   & 96.1 / 96.9 / 99.7 & 77.2 / 85.1 / 98.7 & 69.9 / 75.8 / 90.1 & 68.4 / 74.8 / 90.0 & 67.9 / 75.7 / 87.3 & 65.5 / 71.9 / 86.3 & 43.8 / 52.4 / 75.0 & 24.2 / 29.9 / 42.6 & 10.0 / 13.0 / 17.9 & 2.1 / 4.4 / 8.0 & 0.5 / 1.2 / 1.8   \\
     
     & R2D2   &  98.4 / 98.5 / 99.7 & 84.3 / 91.8 / 98.7 & 86.5 / 91.0 / 97.5 & 83.7 / 87.0 / 97.2 & 86.2 / 89.5 / 97.5 & 83.5 / 87.3 / 96.2 & 76.6 / 82.4 / 93.1 & 58.2 / 66.1 / 83.1 & 31.6 / 37.7 / 49.2 & 19.2 / 22.2 / 27.6 & 13.8 / 15.3 / 18.3  \\
     
     & SuperPoint   &  \textbf{100.0} / \textbf{100.0} / \textbf{100.0} & 99.7 / 99.8 / \textbf{100.0} & 99.7 / 99.7 / \textbf{100.0} & \textbf{100.0} / \textbf{100.0} / \textbf{100.0} & \textbf{99.8} / \textbf{100.0} / \textbf{100.0} & \textbf{99.7} / \textbf{100.0} / \textbf{100.0} & 94.4 / \textbf{99.2} / \textbf{99.5} & \textbf{92.8} / \textbf{96.7} / \textbf{99.7} & \textbf{86.2} / \textbf{90.8} / \textbf{96.1} & \textbf{72.5} / \textbf{78.1} / \textbf{87.2} & \textbf{56.4} / \textbf{60.4} / \textbf{68.1} \\
     
     \bottomrule
     
  \end{tabular}
  }

    \caption{The localization recall rates for the reference paths at illumination levels $k$ with thresholds T1 ($\le$ 0.25m, $\le$2$^\circ$), T2 ($\le$0.50m,$\le$5$^\circ$) and T3 ($\le$5.00m, $\le$10$^\circ$).}
    \label{tab:supplementary_accuracies_full_town01}
    \end{minipage}
\end{table*}

% Illumination - Town10
\begin{table*}[!t]
\subsection{Illumination change results - Town10}
\begin{minipage}[t]{0.48\linewidth}
\centering
   \begin{adjustbox}{width=\linewidth, valign=T}
   \includegraphics[width=1.0\linewidth, trim={0 1cm 0cm 1cm}]{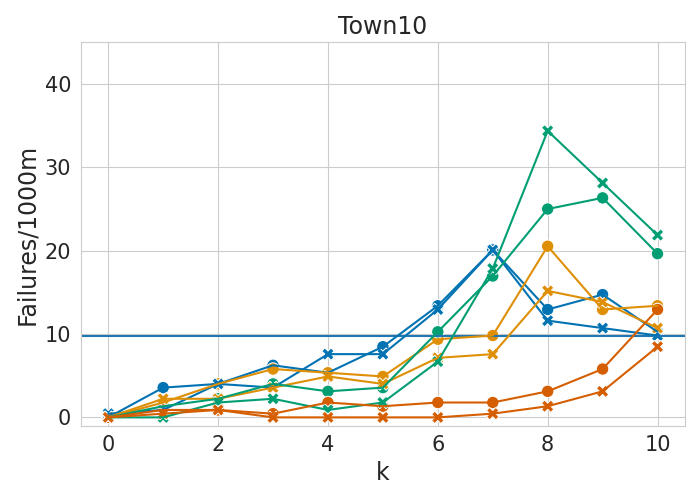}
   \end{adjustbox}
    \captionof{figure}{Relationship of failure rate with illumination levels $k$. Marker color indicates type for local features, shape for global features.}
    \label{fig:supplementary_failure_illumination_town10} %
\end{minipage}%
\hfill
\begin{minipage}[t]{0.48\linewidth}
   \begin{adjustbox}{width=\linewidth, valign=T}
   \includegraphics[width=1.0\linewidth, trim={0 1cm 0cm 1cm}]{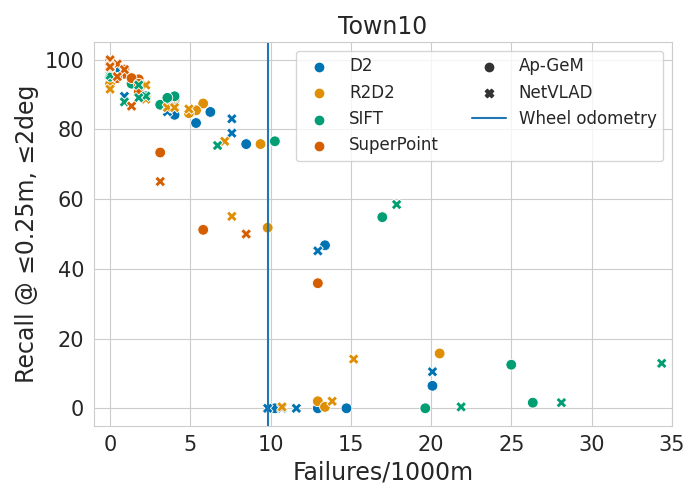}
   \end{adjustbox}
    \captionof{figure}{Relationship between the failure rate and recall rate T1. Marker color and shape indicate feature type.}
    \label{fig:supplementary_failure_recall_illumination_town10}
    \vspace{0.5cm}
\end{minipage}
\vspace{0.5cm}
\hfill
\begin{minipage}[t]{0.75\linewidth}
   \centering
  \begin{adjustbox}{width=\linewidth, valign=T, center}
  \begin{tabular}{l l r r r r r r r r r r r | c }
  &  &   \multicolumn{12}{c}{Town10}       \\
    \cmidrule(lr){3-14}
    %\midrule
     PR & LF &  $k=$
          % town10
     0 & 1 & 2 & 3 & 4 & 5 & 6 & 7 & 8 & 9 & 10 & CT
     \\
    %\midrule
    \midrule
    Ap- & Sift
     %town10
    &     \textbf{0.0} & 1.3 & 2.2 & 4.0 & 3.1 & 3.6 & 10.3 & 17.0 & 25.0 & 26.3 & 19.6
    %Computation time
    & 169 
    \\
     GeM & D2-net
      %town10
    &  \textbf{0.0} & 3.6 & 4.0 & 6.2 & 5.4 & 8.5 & 13.4 & 20.1 & 12.9 & 14.7 & 10.3
    %Computation time
    & 165 
     \\
     & R2D2 
      %town10
    & \textbf{0.0} & 1.8 & 4.0 & 5.8 & 5.4 & 4.9 & 9.4 & 9.8 & 20.5 & 12.9 & 13.4
    %Computation time
    & 194 
     \\
     & SuperPoint 
     %town10
     &  \textbf{0.0} & 0.9 & \textbf{0.9} & 0.4 & 1.8 & 1.3 & 1.8 & 1.8 & 3.1 & 5.8 & 12.9
     %Computation time
    & 193 
     \\
     
    \midrule
    Net- & Sift 
     % town10
    &  \textbf{0.0} & \textbf{0.0} & 1.8 & 2.2 & 0.9 & 1.8 & 6.7 & 17.9 & 34.4 & 28.1 & 21.9
     %Computation time
    & \textbf{134}  
    \\
     VLAD & D2-net 
    % town10
    &  0.4 & 0.9 & 4.0 & 3.6 & 7.6 & 7.6 & 12.9 & 20.1 & 11.6 & 10.7 & 9.8
    & 139 %Computation time
    \\
     & R2D2  
     %town10
     &  \textbf{0.0} & 2.2 & 2.2 & 3.6 & 4.9 & 4.0 & 7.1 & 7.6 & 15.2 & 13.8 & 10.7
      %Computation time
    & 167 
     \\
     %town01
     & SuperPoint
     %town10
     &  \textbf{0.0} & 0.4 & \textbf{0.9} & \textbf{0.0} & \textbf{0.0} & \textbf{0.0} & \textbf{0.0} & \textbf{0.4} & \textbf{1.3} & \textbf{3.1} & \textbf{8.5}
   %Computation time
    & 166  
     \\
     \midrule
     \multicolumn{2}{l}{Wheel odometry} &  \multicolumn{10}{c}{9.8} & &
      \\
     \bottomrule
  \end{tabular}
  \end{adjustbox}
    \caption{Navigation failure rates over 5 repeated runs of the same route at each illumination level $k$. Smaller is better. PR $=$ place recognition method, LF $=$ local feature type, CT $=$ computation time (\textit{ms}).}
    \label{tab:supplementary_failure_illumination_town10}
\end{minipage}
\hfill
\vspace{0.5cm}
\begin{minipage}[t]{\linewidth}
\newcommand\mcat{T1 / T2 / T3}

%\tiny
  \centering
  \resizebox{1.0\linewidth}{!}{
  \begin{tabular}{c c  c c c c c c c c c c c c c c c c c}
  &  & \multicolumn{11}{c}{Town10}   \\
    \cmidrule{3-13}
    \vspace{-0.45cm}
    \\
    \cmidrule{3-13}
    \multirow{2}{*}{PR} & \multirow{2}{*}{LF} &  $k=$ 0 & 1 & 2 & 3 & 4 & 5 & 6 & 7 & 8 & 9 & 10 \\
    \cmidrule{3-13}
    & &   \mcat\  & \mcat\  & \mcat\ & \mcat\ & \mcat\ & \mcat\ & \mcat\ & \mcat\ & \mcat\ & \mcat\ & \mcat\  \\
    %& &   \dcat\ & \dcat\ & \dcat\ & \dcat\ & \dcat\ & \dcat\ & \dcat\ & \dcat\ & \dcat\ & \dcat\ & \dcat\  \\
    \midrule
    Ap- & Sift  & 95.2 /   96.4 /   99.6 & 93.1 /   93.1 /  94.4 & 89.5 /  90.3 /  92.7 & 89.5 /  91.1 /  92.3 & 87.1 /  87.9 /  91.5 & 89.1 /  90.7 /  91.9 & 76.6 /  79.0 /  83.9 & 54.8 /  60.5 /  67.3 & 12.5 /  16.5 /  33.5 & 1.6 /  2.4 /  8.1 & 0.0 /  0.4 /  3.6  \\
    
    GeM & D2-net   & 94.7 /  98.4 /  99.2 & 87.5 /  90.3 /  93.5 & 84.2 /  88.7 /  91.9 & 85.0 /  90.3 /  92.7 & 81.9 /  87.1 /  92.7 & 75.8 /  81.9 /  90.7 & 46.8 /  53.6 /  65.3 & 6.5 /  12.5 /  24.2 & 0.0 /  0.0 /  1.2 & 0.0 /  0.0 /  0.4 & 0.0 /  0.0 /  0.0  \\
     
     & R2D2   & 93.1 /  94.7 /  99.6 & 91.5 /  91.9 /  94.4 & 88.3 /  90.7 /  92.3 & 87.4 /  88.7 /  91.5 & 85.5 /  87.9 /  90.3 & 84.7 /  87.5 /  89.9 & 75.8 /  78.2 /  83.5 & 51.8 /  56.7 /  63.6 & 15.7 /  21.4 /  31.5 & 2.0 /  2.8 /  5.6 & 0.4 /  0.8 /  2.8 \\
     
     & SuperPoint  &  99.6 /  \textbf{100.0} /  \textbf{100.0} & 97.2 /  97.2 /  97.2 & 96.0 /  96.0 /  96.0 & 94.8 /  95.2 /  95.2 & 94.4 /  94.4 /  94.4 & 94.7 /  94.7 /  94.7 & 93.1 /  93.5 /  93.5 & 90.7 /  94.0 /  94.4 & 73.4 /  75.4 /  76.2 & 51.2 /  53.2 /  56.5 & 35.9 /  37.5 /  41.5 \\
   \midrule
    Net & Sift   &  96.4 /  97.2 /  \textbf{100.0} & 95.6 /  96.8 /  98.0 & 92.7 /  94.0 /  94.8 & 89.6 /  91.2 /  93.2 & 87.9 /  90.7 /  93.5 & 89.1 /  91.1 /  92.3 & 75.4 /  77.8 /  85.1 & 58.5 /  63.3 /  68.5 & 12.9 /  17.3 /  35.5 & 1.6 /  4.4 /  9.3 & 0.4 /  0.4 /  2.0  \\
    
    VLAD & D2-net   &  97.2 /  99.6 /  \textbf{100.0} & 89.5 /  91.9 /  96.0 & 86.7 /  89.5 /  94.0 & 85.1 /  89.1 /  94.0 & 83.1 /  88.3 /  92.7 & 78.9 /  85.8 /  90.3 & 45.2 /  58.5 /  69.4 & 10.5 /  14.5 /  28.6 & 0.0 /  0.0 /  0.8 & 0.0 /  0.0 /  0.4 & 0.0 /  0.0 /  0.0  \\
     
     & R2D2   &   91.6 /  92.8 /  99.6 & 92.7 /  94.4 /  96.4 & 88.7 /  91.1 /  92.7 & 86.3 /  89.1 /  91.1 & 85.9 /  89.1 /  90.7 & 86.3 /  89.5 /  91.5 & 76.6 /  80.6 /  87.1 & 55.1 /  59.9 /  66.0 & 14.1 /  20.2 /  33.9 & 2.0 /  2.z8 /  6.5 & 0.4 /  0.8 /  2.0 \\
     
     & SuperPoint   &  \textbf{100.0} /  \textbf{100.0} /  \textbf{100.0} & \textbf{98.8} /  \textbf{99.2} /  \textbf{99.2} & \textbf{97.2} /  \textbf{97.2} /  \textbf{97.6} & \textbf{98.4} /  \textbf{98.8} /  \textbf{98.8} & \textbf{97.6} /  \textbf{98.0} /  \textbf{98.0} & \textbf{98.0} /  \textbf{98.0} /  \textbf{98.0} & \textbf{98.0} /  \textbf{98.0} /  \textbf{98.0} & \textbf{95.2} /  \textbf{96.4} /  \textbf{96.4} & \textbf{86.7} /  \textbf{87.9} /  \textbf{88.7} & \textbf{65.1} /  \textbf{69.5} /  \textbf{72.7} & \textbf{50.0} /  \textbf{55.2} /  \textbf{58.1} \\

     \bottomrule
     
  \end{tabular}
  }

    \caption{The localization recall rates for the reference paths at illumination levels $k$ with thresholds T1 ($\le$ 0.25m, $\le$2$^\circ$), T2 ($\le$0.50m,$\le$5$^\circ$) and T3 ($\le$5.00m, $\le$10$^\circ$).}
    \label{tab:supplementary_accuracies_full_town10}
    \end{minipage}

\end{table*}

% Viewpoint - Town01
\begin{table*}[!t]
\subsection{Viewpoint change results - Town01}
\begin{minipage}[t]{0.48\linewidth}
\centering
    \begin{adjustbox}{width=\linewidth, valign=T}
     \includegraphics[width=1.0\linewidth, trim={0 1.1cm 0cm 1cm}]{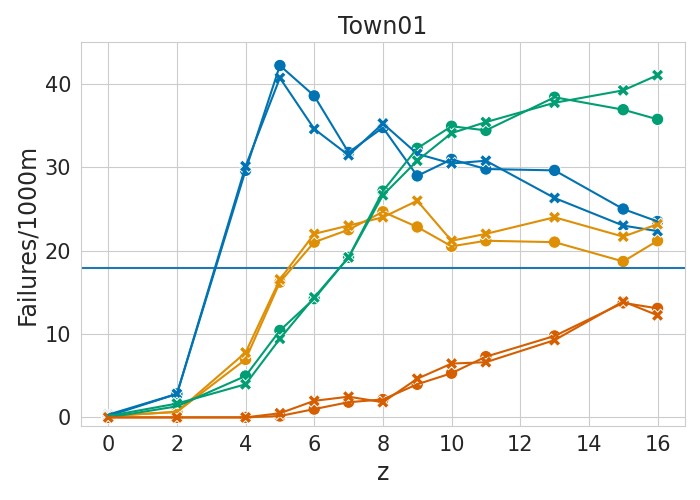}
  \end{adjustbox}
    \captionof{figure}{Relationship between failure rate and elevation and pitch offsets $z,\,\theta$. See Table~\ref{tab:supplementary_failure_pitch_town1} (below) for elevation and pitch pairs.}
    \label{fig:supplementary_failure_pitch_town1} %
\end{minipage}%
\hfill
\begin{minipage}[t]{0.48\linewidth}
    \begin{adjustbox}{width=\linewidth, valign=T}
     \includegraphics[width=1.0\linewidth, trim={0 1.1cm 0cm 1cm}]{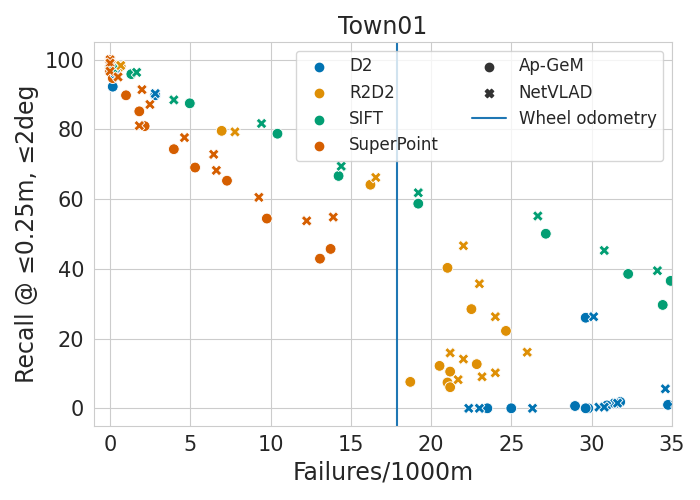}
  \end{adjustbox}
    \captionof{figure}{Relationship between the failure rate and recall rate T1. Marker color and shape indicate feature type.}
    \label{fig:supplementary_failure_recall_pitch_town1}
    \vspace{0.5cm}
\end{minipage}
\vspace{0.5cm}
\hfill
\begin{minipage}[t]{0.75\linewidth}
\centering
 % VIEWPOINT FAILURES

    \centering 
    \resizebox{0.92\linewidth}{!}{ %0.95
  \begin{tabular}{l l r r r r r r r r r r r r r r }
  & & \multicolumn{13}{c}{Town01} &  \\
    \cmidrule{3-15}
    %\midrule
         % town01
     \multirow{2}{*}{PR} & \multirow{2}{*}{LF} &  $z=$ 0 & 2 & 4 & 5 & 6 & 7 & 8 & 9 & 10 & 11 & 13 & 15 & 16 &

     \\

      &  &  $\theta=$ 0 & 10 & 22.5 & 27.5 & 32.5 & 35 & 37.5 & 40 & 40 & 40 & 40 & 40 & 40 &

     \\
    %\midrule
    \midrule
     % town01
    Ap- & Sift & \textbf{0.0} & 1.3 & 5.0 & 10.4 & 14.2 & 19.2 & 27.2 & 32.3 & 34.9 & 34.4 & 38.4 & 36.9 & 35.8 & 

    \\
     % town01
     GeM & D2-net  & 0.2 & 2.8 & 29.6 & 42.2 & 38.6 & 31.8 & 34.8 & 29.0 & 31.0 & 29.8 & 29.6 & 25.0 & 23.5 & 
     \\
      % town01
     & R2D2  & 0.2 & 0.7 & 7.0 & 16.2 & 21.0 & 22.5 & 24.7 & 22.8 & 20.5 & 21.2 & 21.0 & 18.7 & 21.2 & 
     \\
     % town01
     & SuperPoint & \textbf{0.0} & \textbf{0.0} & \textbf{0.0} & \textbf{0.2} & \textbf{1.0} & \textbf{1.8} & 2.2 & \textbf{4.0} & \textbf{5.3} & 7.3 & 9.8 & \textbf{13.7} & 13.1 & 
     \\
     
    \midrule
     % town01
    Net- & Sift  & 0.2 & 1.7 & 4.0 & 9.4 & 14.4 & 19.2 & 26.7 & 30.8 & 34.1 & 35.4 & 37.7 & 39.2 & 41.1 &
    \\
     % town01
     VLAD & D2-net  & 0.3 & 2.8 & 30.1 & 40.7 & 34.6 & 31.5 & 35.3 & 31.6 & 30.5 & 30.8 & 26.3 & 23.0 & 22.4 &
    \\
    %town01
     & R2D2  & 0.2 & 0.7 & 7.8 & 16.6 & 22.0 & 23.0 & 24.0 & 26.0 & 21.2 & 22.0 & 24.0 & 21.7 & 23.2 &
     \\
     %town01
     & SuperPoint  & \textbf{0.0} & \textbf{0.0} & \textbf{0.0} & 0.5 & 2.0 & 2.5 & \textbf{1.8} & 4.6 & 6.5 & \textbf{6.6} & \textbf{9.3} & 13.9 & \textbf{12.3} &
     \\
     \midrule
     \multicolumn{2}{l}{Wheel odometry} &  \multicolumn{12}{c}{17.9} %& 17.9 &  &  &  & &  &  &  &  &  &  &  &  
      \\
     \bottomrule
  \end{tabular} %\resizebox{0.33\linewidth}{!}{
  }
  
%  \hfill% 
  %%%%%%%%%%%%%%%%%%%%%%%%
  % BEGIN WEATHER RESULTS
  %%%%%%%%%%%%%%%%%%%%%%%%
%  \begin{minipage}[t]{0.31\linewidth}
%  \captionof{table}{Failure rates at gallery-to-query weather (visibility) changes $v$.}%
%    \centering
    %\captionof{table}{Blalbla}
%    \resizebox{0.95\linewidth}{!}{ % 1.0
%  \begin{tabular}{l l r r r r }
%   & &\multicolumn{4}{c}{Town01}  \\
%    \cmidrule{3-6}
    %\midrule
         % town01
%    PR & LF & $v=$ 90 & 60 & 30 & 10 

%     \\
    %\midrule
%    \midrule
     % town01
%    Ap- & Sift &  8.5 & 25.4 & 25.4 & 21.9  

%    \\
     % town01
%    GeM & D2-net  & 12.1 & 13.8 & 10.3 & 12.9 
%     \\
      % town01
%     & R2D2  & 10.3 & 12.5 & 10.3 & 10.3 
%     \\
     % town01
%     & SuperPoint & \textbf{0.0} & 0.4 & 1.8 & 2.2 
%     \\
     
 %   \midrule
     % town01
%    Net- & Sift  & 7.6 & 25.9 & 29.5 & 25.9 
%    \\
     % town01
%     VLAD & D2-net  & 12.5 & 13.4 & 10.7 & 9.4
%    \\
    %town01
%     & R2D2  & 9.4 & 8.0 & 7.6 & 8.5  
%     \\
     %town01
%     & SuperPoint  & \textbf{0.0} & \textbf{0.0} & \textbf{0.0} & \textbf{0.9} 
%     \\
%     \midrule
%     \multicolumn{2}{l}{Wheel odometry}  & \multicolumn{4}{c}{9.8} %& 9.8 &  &  &  
%      \\
%     \bottomrule
%  \end{tabular}
%  }
%  \label{tab:weather_failures}
%  \end{minipage}
     \captionof{table}{Navigation failure rates over 5 repetitions of the same route at each gallery to-query camera pose (viewpoint) offset. $z=$ elevation shift, $\theta=$ pitch shift.}
    \label{tab:supplementary_failure_pitch_town1}
\end{minipage}
\hfill
\vspace{0.5cm}
\begin{minipage}[t]{\linewidth}
\centering
\newcommand\mcat{T1 / T2 / T3}

%\tiny
  \centering
  \resizebox{1.0\linewidth}{!}{
  \begin{tabular}{l l r r r r r r r r r r r r r r }
  & & \multicolumn{13}{c}{Town01} &  \\
    \cmidrule{3-15}
    \vspace{-0.45cm}
    \\
    \cmidrule{3-15}
    %\midrule
         % town01
     \multirow{2}{*}{PR} & \multirow{2}{*}{LF} &  $z=$ 0 & 2 & 4 & 5 & 6 & 7 & 8 & 9 & 10 & 11 & 13 & 15 & 16 &

     \\

      &  &  $\theta=$ 0 & 10 & 22.5 & 27.5 & 32.5 & 35 & 37.5 & 40 & 40 & 40 & 40 & 40 & 40 & \\
    \midrule
    & &   \mcat\  & \mcat\  & \mcat\ & \mcat\ & \mcat\ & \mcat\ & \mcat\ & \mcat\ & \mcat\ & \mcat\ & \mcat\ & \mcat\ & \mcat\  \\
    %& &   \dcat\ & \dcat\ & \dcat\ & \dcat\ & \dcat\ & \dcat\ & \dcat\ & \dcat\ & \dcat\ & \dcat\ & \dcat\ & \dcat\ & \dcat\  \\
    \midrule
    Ap- & Sift  & 98.0 / 98.2 / 99.8 & 95.9 / 96.9 / 97.9 & 87.5 / 89.3 / 93.1 & 78.8 / 83.4 / 88.3 & 66.7 / 72.1 / 78.8 & 58.7 / 65.8 / 74.0 & 50.1 / 57.8 / 65.7 & 38.6 / 47.1 / 55.8 & 36.6 / 41.5 / 49.2 & 29.7 / 38.4 / 46.3 & 21.4 / 26.5 / 33.3 & 17.8 / 21.9 / 31.2 & 17.4 / 22.2 / 29.7  \\
    
     GeM & D2-net   & 92.3 / 95.7 / 99.8 & 89.8 / 95.2 / 98.2 & 26.0 / 46.4 / 76.8 & 10.3 / 21.8 / 53.9 & 4.1 / 9.5 / 23.5 & 1.8 / 8.2 / 21.2 & 1.0 / 3.8 / 13.5 & 0.7 / 2.3 / 8.7 & 0.8 / 1.3 / 8.1 & 0.0 / 0.3 / 5.6 & 0.0 / 0.2 / 2.3 & 0.0 / 0.0 / 1.0 & 0.0 / 0.0 / 0.5  \\
     
     & R2D2   & 98.0 / 98.4 / \textbf{100.0} & 98.0 / 98.0 / 98.5 & 79.6 / 81.4 / 88.8 & 64.1 / 67.6 / 75.5 & 40.3 / 49.7 / 59.9 & 28.5 / 38.5 / 50.2 & 22.2 / 29.9 / 44.1 & 12.7 / 21.2 / 36.0 & 12.2 / 20.2 / 31.7 & 10.5 / 18.3 / 28.6 & 7.4 / 14.8 / 22.9 & 7.6 / 13.0 / 21.1 & 6.1 / 11.5 / 21.1 \\
     
     & SuperPoint  & \textbf{100.0} / \textbf{100.0} / \textbf{100.0} & \textbf{99.5} / \textbf{99.5} / \textbf{99.7} & \textbf{96.7} / \textbf{96.7} / \textbf{98.5} & 94.7 / 94.9 / \textbf{97.4} & 89.8 / 90.3 / 94.1 & 85.2 / 86.8 / 92.4 & 81.0 / 83.3 / 88.2 & 74.3 / 76.6 / 83.9 & 69.1 / 72.7 / 80.1 & 65.3 / 70.1 / 76.0 & 54.4 / 60.7 / 66.4 & 45.7 / 52.3 / 57.1 & 42.9 / 49.8 / 54.9  \\
   \midrule
    Net- & Sift   & 97.4 / 98.5 / 99.8 & 96.4 / 96.9 / 97.9 & 88.5 / 90.1 / 93.8 & 81.7 / 85.2 / 89.3 & 69.5 / 75.5 / 82.9 & 61.8 / 67.3 / 73.5 & 55.2 / 61.1 / 68.6 & 45.3 / 52.2 / 63.3 & 39.5 / 46.9 / 55.1 & 38.6 / 44.7 / 52.2 & 26.5 / 33.8 / 43.8 & 23.6 / 27.8 / 36.6 & 20.1 / 23.9 / 30.8   \\
    
     VLAD & D2-net   &  96.1 / 96.9 / 99.7 & 90.3 / 96.7 / 98.7 & 26.3 / 46.6 / 78.5 & 12.3 / 21.2 / 57.2 & 5.6 / 11.3 / 28.2 & 1.5 / 7.4 / 23.0 & 1.2 / 4.8 / 16.8 & 1.5 / 3.0 / 14.1 & 0.3 / 1.3 / 8.9 & 0.3 / 0.8 / 5.9 & 0.0 / 0.0 / 3.3 & 0.0 / 0.0 / 1.3 & 0.0 / 0.0 / 1.6  \\
     
     & R2D2   &  98.4 / 98.5 / 99.7 & 98.4 / 98.4 / 99.0 & 79.3 / 81.1 / 88.7 & 66.2 / 70.8 / 79.3 & 46.6 / 53.5 / 63.4 & 35.7 / 44.1 / 53.3 & 26.3 / 33.3 / 45.5 & 16.1 / 25.6 / 38.6 & 15.9 / 23.0 / 33.4 & 14.1 / 19.0 / 29.2 & 10.2 / 17.2 / 23.8 & 8.2 / 12.6 / 21.2 & 9.0 / 12.8 / 20.2  \\
     
     & SuperPoint   & \textbf{100.0} / \textbf{100.0} / \textbf{100.0} & 99.0 / 99.0 / 99.2 & \textbf{96.7} / \textbf{96.7} / 98.0 & \textbf{95.1} / \textbf{95.1} / \textbf{97.4} & \textbf{91.4} / \textbf{92.3} / \textbf{96.2} & \textbf{87.2} / \textbf{88.3} / \textbf{95.1} & \textbf{81.1} / \textbf{84.9} / \textbf{91.4} & \textbf{77.7} / \textbf{81.1} / \textbf{88.3} & \textbf{72.9} / \textbf{77.0} / \textbf{84.5} & \textbf{68.3} / \textbf{73.8} / \textbf{79.4} & \textbf{60.5} / \textbf{68.3} / \textbf{73.7} & \textbf{54.9} / \textbf{66.1} / \textbf{71.3} & \textbf{53.8} / \textbf{62.0} / \textbf{68.1}  \\
     
     \bottomrule
     
  \end{tabular}
  }

    \caption{The localization recall rates for the reference paths at elevation and pitch changes $z,\,\theta$ with thresholds T1 ($\le$ 0.25m, $\le$2$^\circ$), T2 ($\le$0.50m,$\le$5$^\circ$) and T3 ($\le$5.00m, $\le$10$^\circ$).}
    \label{tab:supplementary_failure_recall_pitch_town1}
\end{minipage}

\end{table*}

%Weather - Town10
\begin{table*}[!t]
\subsection{Weather change results - Town10}
\begin{minipage}[t]{0.48\linewidth}
\centering
    \begin{adjustbox}{width=\linewidth, valign=T}
     \includegraphics[width=1.0\linewidth, trim={0 1.1cm 0cm 1cm}]{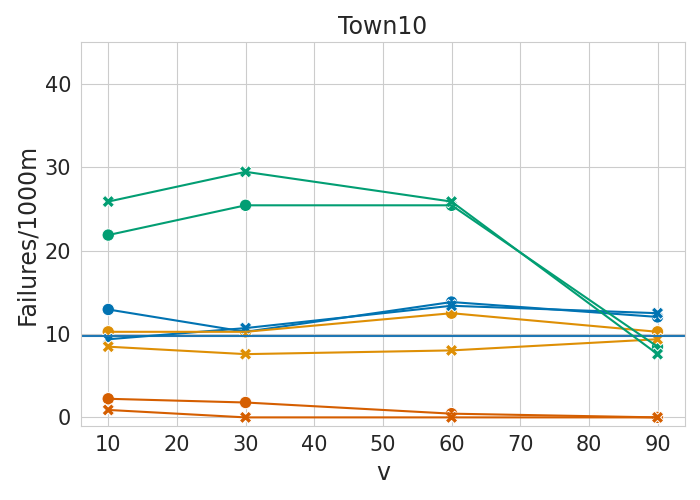}
  \end{adjustbox}
    \captionof{figure}{Relationship between failure rate and visual range $v$.}
    \label{fig:supplementary_failure_weather_town10} %
\end{minipage}%
\hfill
\begin{minipage}[t]{0.48\linewidth}
    \begin{adjustbox}{width=\linewidth, valign=T}
     \includegraphics[width=1.0\linewidth, trim={0 1.1cm 0cm 1cm}]{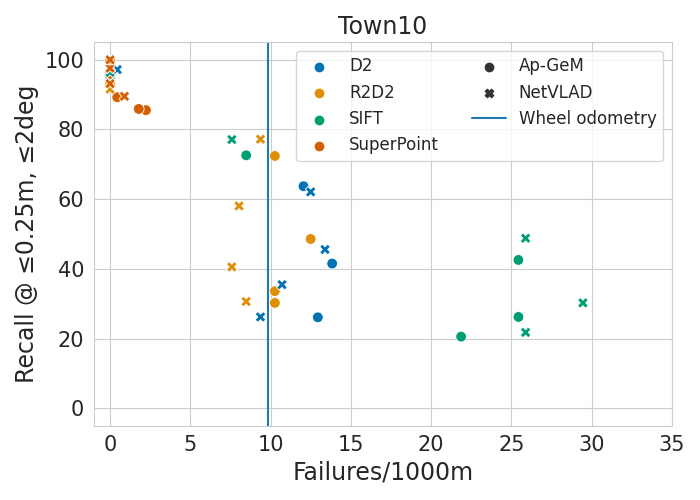}
  \end{adjustbox}
    \captionof{figure}{Relationship between the failure rate and recall rate T1. Marker color and shape indicate feature type.}
    \label{fig:supplementary_failure_recall_weather_town10}
    \vspace{0.5cm}
\end{minipage}
\vspace{0.5cm}
\hfill
\begin{minipage}[t]{\linewidth}
\centering
 \centering
    %\captionof{table}{Blalbla}
  \begin{tabular}{l l r r r r }
   & &\multicolumn{4}{c}{Town10}  \\
    \cmidrule{3-6}
    %\midrule
         % town01
    PR & LF & $v=$ 90 & 60 & 30 & 10 

     \\
    %\midrule
    \midrule
     % town01
    Ap- & Sift &  8.5 & 25.4 & 25.4 & 21.9  

    \\
     % town01
    GeM & D2-net  & 12.1 & 13.8 & 10.3 & 12.9 
     \\
      % town01
     & R2D2  & 10.3 & 12.5 & 10.3 & 10.3 
     \\
     % town01
     & SuperPoint & \textbf{0.0} & 0.4 & 1.8 & 2.2 
     \\
     
    \midrule
     % town01
    Net- & Sift  & 7.6 & 25.9 & 29.5 & 25.9 
    \\
     % town01
     VLAD & D2-net  & 12.5 & 13.4 & 10.7 & 9.4
    \\
    %town01
     & R2D2  & 9.4 & 8.0 & 7.6 & 8.5  
     \\
     %town01
     & SuperPoint  & \textbf{0.0} & \textbf{0.0} & \textbf{0.0} & \textbf{0.9} 
     \\
     \midrule
     \multicolumn{2}{l}{Wheel odometry}  & \multicolumn{4}{c}{9.8} %& 9.8 &  &  &  
      \\
     \bottomrule
  \end{tabular}
    \caption{Failure rates at gallery-to-query weather (visibility) changes $v$.}
    \label{tab:supplementary_failure_weather_town10}
\end{minipage}
\vspace{0.5cm}
\hfill
\begin{minipage}[t]{0.7\linewidth}
\centering
 \newcommand\mcat{T1 / T2 / T3}

%\tiny
  \centering
  \resizebox{1.0\linewidth}{!}{
  \begin{tabular}{l l r r r r }
  & & \multicolumn{4}{c}{Town10}  \\
    \cmidrule{3-6}
    \vspace{-0.45cm}
    \\
    \cmidrule{3-6}
    %\midrule
         % town01
     PR & LF &  $v=$ 90 & 60 & 30 & 10 & 
    \midrule
    & &   \mcat\  & \mcat\  & \mcat\ & \mcat\  \\
    %& &   \dcat\ & \dcat\ & \dcat\ & \dcat\  \\
    \midrule
    Ap- & Sift  &  72.6 / 79.0 / 86.3 & 42.6 / 43.0 / 49.0 & 26.2 / 28.2 / 31.5 & 20.6 / 23.4 / 28.2 \\
    
     GeM & D2-net   & 63.7 / 71.0 / 81.5 & 41.5 / 44.4 / 54.8 & 30.2 / 33.1 / 40.3 & 26.1 / 29.7 / 35.3 \\
     
     & R2D2   & 72.4 / 76.8 / 82.8 & 48.6 / 51.4 / 56.3 & 33.6 / 36.8 / 40.9 & 30.2 / 31.5 / 34.3 \\
     
     & SuperPoint  & 96.0 / 96.4 / 96.4 & 89.2 / 90.0 / 90.0 & 85.9 / 86.7 / 88.7 & 85.5 / 86.7 / 87.6 \\
   \midrule
    Net- & Sift   & 77.1 / 82.3 / 88.8 & 48.8 / 51.6 / 56.5 &  30.2 / 34.3 / 37.9 & 21.8 / 23.4 / 28.2 \\
    
     VLAD & D2-net   &  62.1 / 70.6 / 82.3 & 45.6 / 50.8 / 63.3 & 35.5 / 37.1 / 44.0 & 26.2 / 31.5 / 39.1 \\
     
     & R2D2   & 77.2 / 81.2 / 86.8 & 58.1 / 59.7 / 64.1 &   40.6 / 42.2 / 46.6 & 30.6 / 34.7 / 39.5 \\
     
     & SuperPoint   & \textbf{97.6} / \textbf{97.6} / \textbf{97.6} &\textbf{97.6} / \textbf{97.6} / \textbf{97.6} & \textbf{93.1} / \textbf{94.0} / \textbf{94.0} & \textbf{89.5} / \textbf{90.7} / \textbf{91.5} \\
     
     \bottomrule
     
  \end{tabular}
  }
    \caption{The localization recall rates for the reference paths at visual ranges $v$ with thresholds T1 ($\le$ 0.25m, $\le$2$^\circ$), T2 ($\le$0.50m,$\le$5$^\circ$) and T3 ($\le$5.00m, $\le$10$^\circ$).}
    \label{tab:supplementary_failure_recall_weather_town10}
\end{minipage}
\hfill
\vspace{0.5cm}
\end{table*}
